# Supplementary material for: 007: Democratically Finding The Cause of Packet Drops
Source: arXiv:1802.07222 source file (2018-02-20)
Supplement: Supplementary file 1 [file appendix.tex]

\section{Proof of optimality of Eq. 1}
	\label{sec:optimality}

\begin{theorem}

Consider a network with no lines, i.e., a network in which there are no paths between two non-adjacent nodes that involve the same links. Explicitly, for every pair of nodes~$v,w$ that are not neighbors~$\bigcap_{c \in \calP(v,w)} c = \emptyset$, where $\calP(v,w)$ is the set of all paths between the nodes~$v,w$. Let~$\calF$ be the set of links in this network that failed by dropping at least one packet and~$\phi^o$ be a solution of
\begin{equation}\label{P:setCover}
\begin{aligned}
	\text{minimize}&
		&&\abs{\phi}
	\\
	\text{subject to}&
		&&\norm{A_{\phi} \cdot \ones}_0 = \abs{\calC}
\end{aligned}
\end{equation}
If~$\calC$ contains every path involving the links in~$\calF$, $\phi^o = \calF$.

%Furthermore, if for all~$\ell \in \calF$ there exists \emph{at least} one connection in~$\calC$ impacted by~$\ell$---i.e., $\forall \ell \in \calF$, $\exists\ c \in \calC$ such that $\ell \cap c = \ell$---then $\phi^o = \calF$.

\end{theorem}

\begin{proof}

Start by showing that any solution~$\phi^o$ of Problem~\ref{P:setCover} is such that~$\abs{\phi^o} \leq \abs{\calF}$. Indeed, suppose it is not. Then~$\calF$, which satisfies the constraint, is such that~$\abs{\calF} < \abs{\phi^o}$, contradicting the optimality of~$\phi^o$.

Next, suppose there exist~$\phi^\prime$ such that~$\abs{\phi^\prime} < \abs{\calF}$. We show that $\phi^\prime$ cannot be feasible. Indeed, take any~$\ell \in \calF$ and~$\ell \notin \phi^\prime$. If there exist a path in~$\calC$ that contains only~$\ell$, then~$\phi^\prime$ cannot be feasible.

%If this is not the case, recall that~$\calC$ contains every path involving~$\ell$ and that all that go through~$\ell$ cannot go through the same links.

\texttt{Need to show: there exists a path~$c \in \calC$ which contains $\ell$ and does not contain any link in~$\phi^\prime$?}

\end{proof}

\section{Proof of theorem 1}
	\label{sec:proof1}

\begin{theorem}\label{theorem1}

Let hosts under a top of the rack switch~(ToR) communicate with hosts under a different ToR uniformly at random. Then, in a data center with a Clos topology, the rate of ICMP~packets generated by any switch due to a traceroute from~\Sys is below~$T_{max}$ if the connection rate~$C$ of each host is upper bounded as in
\begin{align}\label{eq:maxC}
	C \leq \frac{
		n_1 n_2 T_{max}
	}{
		H \max\left[ n_2, \frac{n_0^2(\npod-1)}{n_0 \npod-1} \right]
	}
		\text{,}
\end{align}
where~$n_0$, $n_1$, and $n_2$ are the numbers of ToR, $T_1$, and~$T_2$ switches respectively and~$H$ is the number of hosts under each ToR.

\end{theorem}

\begin{proof}

\Sys only instantiates traceroutes for a connection if it experiences at least one retransmission. Let~$p$ denote the probability that a connection experiences a retransmission. Then, the rate of traceroutes that will go through any level~1 link is given by~$R_1 = \frac{1}{n_1} CHp$ and through any level~2 link is~$R_2 = \frac{n_0}{n_1n_2}\frac{n_0(n_{pod}-1)}{n_0n_{pod}-1)} CHp$. Using the fact that these rates are maximized for~$p = 1$, we obtain~\eqref{eq:maxC} by making~$\max \left[ R_1,R_2 \right] \leq T_\text{max}$.

\end{proof}

\section{Proof of theorem 3}
	\label{sec:proof3}

\begin{theorem}\label{T:vigilWorks}

In a Clos topology with~$\npod \geq \frac{n_0}{n_1} + 1$, \Sys will find with probability~$1-2e^{-\calO(N)}$ the set of~$k < \frac{n_2 (n_0 \npod - 1)}{n_0 (\npod - 1)}$ bad links that fail with probability~$p_b$ among good links that fail with probability~$p_g$ if $p_b \ge \alpha p_g$, where $N$ is the total number of connections between hosts and
\begin{equation}\label{eq:alpha}
	\alpha =
	\frac{
		n_0 (4 n_0 - k) (\npod - 1)
	}{
		n_2 (n_0 \npod - 1) - n_0 (\npod - 1) k
	}
\end{equation}

\end{theorem}

\begin{proof}

Take~$s_b$ to be the \emph{probability of a bad link scoring} and~$s_g$ to be the \emph{probability of a good link scoring}. The proof then relies on the following two lemmas:

\begin{lemma}\label{T:whp}
If $s_b \geq s_g$, \Sys will find all bad links with probability $1-2e^{-\calO(N)}$.
\end{lemma}

\begin{lemma}\label{T:scoringProb}
In a Clos topology with $\npod \geq \frac{n_0}{n_1} + 1$ and for~$k < n_0$ bad links,
\begin{subequations}\label{eq:scoringProb}
\begin{align}
	s_b &\geq \frac{p_b}{n_0 n_1 \npod}
		\label{eq:badScoringProb}
	\\
	s_g &\leq
	\frac{1}{n_1 n_2 \npod}
	\frac{n_0 (\npod - 1)}{n_0 \npod - 1}
	\left[
		4 p_g + \frac{k}{n_0} (p_b - p_g)
	\right]
		\label{eq:goodScoringProb}
\end{align}
\end{subequations}
\end{lemma}

Let us defer the proofs of these Lemmas and proceed to see how they imply Theorem~\ref{T:vigilWorks}. Indeed, from the bounds in~\eqref{eq:scoringProb} it holds that
\begin{multline*}
	\text{\eqref{eq:badScoringProb}}
	\geq
	\text{\eqref{eq:goodScoringProb}}
	\Rightarrow
	\\	
	p_b
	\geq
	\underbrace{
		\left[
			1 - \frac{n_0 (\npod - 1) k}{n_2 (n_0 \npod - 1)}
		\right]^{-1}
		\frac{n_0 (4 n_0 - k) (\npod - 1)}{n_2 (n_0 \npod - 1)}
	}_\alpha
	p_g
	\\
	\Rightarrow
	s_b \geq s_g
		\text{,}
\end{multline*}
which is informative only when~$\frac{n_0 (\npod - 1) k}{n_2 (n_0 \npod-1)} < 1$~(otherwise~$\alpha < 0$). Thus, $p_b \geq \alpha p_g \Rightarrow s_b \geq s_g$ for~$\alpha$ as in~\eqref{eq:alpha}, which from Lemma~\ref{T:whp} implies that~\Sys will give higher scores to bad links than good links with high probability.

In the sequel, we provide sketches of the proofs of Lemmas~\ref{T:whp} and~\ref{T:scoringProb}

%%%%%%%%%%%%%%%%% PROOF OF LEMMA 1 %%%%%%%%%%%%%%%%%
\begin{proof}[Proof sketch of Lemma~\ref{T:whp}]

The score of a bad~(good) link is a binomial random variable~$B$~($G$) with parameters~$N$, the total number of connections, and~$s_b$~($s_g$), the probability of a bad~(good) link scoring. Vigil will rank bad links above good links as long as~$B \geq G$, i.e., the score of bad links is larger than the score of good links. This event contains $\{G \leq (1+\delta) N s_g \cap B \geq (1-\delta) N s_b\}$ for~$\delta \leq \frac{s_b - s_g}{s_b + s_g}$, so that the probability of Vigil correctly identifying the bad links is bounded by
\begin{align}
	\Pr(B \geq G) &\geq
	\Pr\left[ G \leq (1+\delta) N s_g \cap
				B \geq (1-\delta) N s_b \right]
	\notag\\\label{E:pBound}
	{}&\geq 1 - \epsilon
		\text{,}
\end{align}
with $\epsilon = \Pr\left[ G \geq (1+\delta) N s_g \right] + \Pr\left[ B \leq (1-\delta) N s_b \right]$. The last inequality holds from the Boole-Fréchet inequalities. Using the large deviation principle, the probabilities in $\epsilon$ can be bounded by
$\Pr\left[ G \geq (1+\delta) N s_g \right] \leq
	e^{-N \DKL((1+\delta) s_g \| s_g)}$ and
$\Pr\left[ G \geq (1+\delta) N s_g \right] \leq
	e^{-N \DKL((1+\delta) s_g \| s_g)}$,
where we denote by $\DKL(p \| q )$ the Kullback-Leibler divergence between two Bernoulli distributions with probabilities of success~$p$ and~$q$~\cite{ldp}. Using Pinsker's inequality to obtain that $\DKL(p \| q) \geq 2 \abs{p - q}^2$~\cite{infotheory} and the fact that~$s_b \geq s_g$, we get from~\eqref{E:pBound} that
\begin{equation*}
	\Pr(B_N \geq G_N) \geq
		1 - 2 e^{-2 N \delta^2 s_g^2} = 1 - 2 e^{-\calO(N)}
		\text{.}
		\qedhere
\end{equation*}
\end{proof}
%%%%%%%%%%%%%%%%% END OF PROOF OF LEMMA 1 %%%%%%%%%%%%%%%%%

\begin{proof}[Proof sketch of Lemma~\ref{T:scoringProb}]

The inequality~\eqref{eq:badScoringProb} is straightforward to obtain by observing that the probability of a bad link scoring is larger than the probability of it dropping a packet. Moreover, since~$n_2 \leq n_0$, the probability of a connection being routed through a level~1 link is smaller than a level~2 link. Therefore, the lower bound in~\eqref{eq:badScoringProb} is given by the probability of a connection going through a level~1 link and that link dropping a packet.

In the case of~\eqref{eq:goodScoringProb}, we decompose the event of a failure as a union of event and use the union bound~$\Pr[\cup A_i] \leq \sum \Pr[A_i]$. Note that since the probability of being routed through a level~2 link is larger, suffices to find a bound in this case. Thus, a good level~2 link scores if a connection goes through the link \emph{and} (i)~the link drops the packet; or (ii)~the connection also goes through some level~1 link in the same pod and this link drops the packet; or (iii)~the connection also goes through some level~2 in another pod and this link drops the packet; or (iv)~the connection also goes through some level~1 link in another pod and this link drops the packet. Using the union bound then gives
\begin{align*}
	s_g \leq
	\Pr[\bB_0]
	\left\{ \vphantom{\frac{1}{n_0}} \right.
		p_g
		&+
		\frac{1}{n_0}
			\left[ k_2 p_b + (n_0 - k_2) p_g \right]
		\\
		{}&+
		\frac{
			k_3 p_b + \left[ n_1 (\npod - 1) - k_3 \right] p_g
		}{
			n_1 (\npod - 1)
		}
		\\
		{}&+
		\frac{
			k_4 p_b + (n_0 n_1 (\npod - 1) - k_4) p_g
		}{
			n_0 n_1 (\npod - 1)
		}
	\left. \vphantom{\frac{1}{n_0}} \right\}
		\text{,}
\end{align*}
where $\Pr[\bB_0] = \frac{n_0 (\npod - 1)}{\npod n_1 n_2 (n_0 \npod - 1)}$ and~$k_2$, $k_3$, and~$k_4$ are the number of failed links under conditions~(ii), (iii), and~(iv) respectively. Since~$\npod \geq \frac{n_0}{n_1} + 1$, the second term has the largest coefficient and given that the number of failed links is less than~$n_0$, the bound in~\eqref{eq:goodScoringProb} holds when all failed links are under condition~(ii), i.e., $k_2 = k$, $k_3 = 0$, and~$k_4 = 0$. \qedhere

\end{proof}

\end{proof}
